# Supplementary material for: Non-linear fluctuating hydrodynamics for KPZ scaling in isotropic spin chains
Source: arXiv:2212.03696 source file (2023-08-01)
Supplement: Supplementary file 1 [file SM.pdf]

# Non-linear fluctuating hydrodynamics for KPZ scaling in isotropic spin chains

Jacopo De Nardis,<sup>1</sup> Sarang Gopalakrishnan,<sup>2</sup> and Romain Vasseur<sup>3</sup>

<sup>1</sup>*Laboratoire de Physique Théorique et Modélisation, CNRS UMR 8089,  
CY Cergy Paris Université, 95302 Cergy-Pontoise Cedex, France*

<sup>2</sup>*Department of Electrical and Computer Engineering,  
Princeton University, Princeton, NJ 08544, USA*

<sup>3</sup>*Department of Physics, University of Massachusetts, Amherst, MA 01003, USA*

## INVARIANCE OF THE GAUSSIAN MEASURE UNDER COUPLED KPZ EQUATIONS

We here show that Gaussian measure

$$P = Z^{-1} \exp \left( -\frac{1}{2\chi} \int dx [(\partial_x h_m)^2 + (\partial_x h_\phi)^2] \right), \quad (1)$$

is stationary under the coupled KPZ equations

$$\partial_t h_m + \kappa \partial_x h_m \partial_x h_\phi = D_m \partial_x^2 h_m + \xi_m, \quad (2)$$

$$\partial_t h_\phi + \frac{\kappa}{2} (\partial_x h_m)^2 = D_\phi \partial_x^2 h_\phi + \xi_\phi, \quad (3)$$

where we have introduced the height fields  $m(x, t) = \partial_x h_m$  and  $\phi(x, t) = \partial_x h_\phi$ . The stationary measure of those equations satisfies

$$\sum_{i=m,\phi} \int dx \frac{\delta}{\delta h_i(x)} \left( -D_i \partial_x^2 h_i + G_i^{kl} (\partial_x h_k) (\partial_x h_l) + \frac{1}{2} \frac{\delta}{\delta h_i(x)} \right) P = 0, \quad (4)$$

where  $G_m^{\phi\phi} = G_m^{\phi m} = \kappa/2$ ,  $G_\phi^{mm} = \kappa/2$  characterize the non-linear terms in (2). This equation relates the strength of the noise and dissipation to the susceptibility  $\chi$ , which we solve by setting  $D_m = D_\phi = 1$  and taking the noise to have unit strength so that  $\chi = 1/2$ . Meanwhile, the nonlinear terms lead to the condition

$$\int dx \left( \frac{\delta}{\delta h_m(x)} [\kappa (\partial_x h_m) (\partial_x h_\phi)] P + \frac{\delta}{\delta h_\phi(x)} \left[ \frac{\kappa}{2} (\partial_x h_m)^2 \right] \right) P = 0, \quad (5)$$

which is satisfied by the Gaussian measure since

$$-\kappa \int dx [(\partial_x h_m) (\partial_x h_\phi)] \partial_x^2 h_m - \frac{\kappa}{2} \int dx [(\partial_x h_m)^2] \partial_x^2 h_\phi = -\frac{\kappa}{2} \int dx \frac{\partial}{\partial x} [(\partial_x h_m)^2 \partial_x h_\phi] = 0, \quad (6)$$

up to boundary terms.

## DERIVATION OF THE NLFH EQUATIONS FROM GHD

Let us start by deriving the first equation for the magnetization  $m$  in the Heisenberg chain at Euler scale

$$\partial_t m(x, t) + \kappa \partial_x (m(x, t) \phi(x, t)) = 0. \quad (7)$$

From GHD, we have the following equation at Euler scale for the magnetization

$$\partial_t m(x, t) + \partial_x (m(x, t) v_\infty^{\text{eff}}(x, t)) = 0. \quad (8)$$

The quantity  $v_\infty^{\text{eff}} = \lim_{s \rightarrow \infty} v_s^{\text{eff}}$  depends non-trivially on the global equilibrium state, specified by chemical potentials  $\{\beta^i\}_i$  (in general there is an infinite number of them, as the model is integrable) via the thermodynamic Bethe ansatz

dressing, and it is zero for any finite temperature equilibrium state. We consider therefore a small, space dependent, perturbation around a (infinite) temperature state  $\beta^i = \beta \delta_{i,1}$ , namely, using repeated indices convention,

$$v_\infty^{\text{eff}}(\beta + \delta\beta^i) = \delta\beta^i \frac{\partial v_\infty^{\text{eff}}}{\partial \beta^i} = \frac{\partial v_\infty^{\text{eff}}}{\partial n_j} \delta n_j, \quad (9)$$

where we used the collective index  $j$  to denote strings  $s$  and momenta  $u$ . We have introduced the filling functions  $n_s(u)$  characterizing the equilibrium state with generic chemical potentials, so that we have  $n_j(\beta_0^i + \delta\beta^i) = n_j + \delta n_j$ , with  $\delta n_j = (\partial n_j / \partial \beta^i) \delta \beta^i$ . Moreover, the total densities of states  $k'_s(u) = 2\pi \rho_s^{\text{tot}}(u)$  and the velocities are  $v_s^{\text{eff}}(u)$ , for each type  $s$  of quasiparticle. This also allows us to define the dressing operation  $f^{\text{dr}} = (1 - Tn)^{-1}f$  as a linear operation on any (integrable) function, in terms of the scattering shift  $T_{s,s'}(u, u')$  of the model. From generic dressing relations, see for example [1], we have, with  $\chi$  the spin susceptibility,

$$\delta f_j^{\text{dr}} = T_{j,j'}^{\text{dr}} f_{j'}^{\text{dr}} \delta n_j, \quad \delta v_\infty^{\text{eff}} = -\frac{v_j^{\text{eff}} \rho_j^{\text{tot}} \mu_j^{\text{dr}}}{2\chi} \delta n_j. \quad (10)$$

Here, the dressed magnetic moment is obtained as the low field limit of the dressed magnetization  $\mu_j^{\text{dr}} = \lim_{h \rightarrow 0+} m_j^{\text{dr}}/h$ , where  $h$  is a global magnetic field, but also from the large  $s$  limit of the dressed scattering kernel  $\mu_s^{\text{dr}}/(2\chi) = -\lim_{s' \rightarrow \infty} T_{s',s}^{\text{dr}}/\rho_{s'}^{\text{tot}}$  and  $\lim_{s \rightarrow \infty} T_{s,s'}^{\text{dr}} = -2m_{s'}^{\text{dr}}/\pi$  [2]. Notice that since the velocities  $v_j^{\text{eff}}$  on an equilibrium state are all odd functions of  $u$ , the only modifications that give non-zero contributions are the antisymmetric in momenta  $u$ . Therefore we can write, restoring summation over  $s$  and integration over  $u$ :

$$\delta v_\infty^{\text{eff}} = \frac{-1}{2\chi} \sum_s \int_0^\infty du \left[ \rho_s^{\text{tot}}(u) v_s^{\text{eff}}(u) \mu_s^{\text{dr}} \right]_\beta [\delta n_s(u) - \delta n_s(-u)], \quad (11)$$

where the block  $[\cdot]_\beta$  is evaluated at finite (or infinite) temperature and is a functional of the global equilibrium state. We now proceed as in the main text: we neglect the fluctuations of quasiparticles  $\delta n_s$  for small  $s$  (as they spread ballistically and decouple at large times), and we only consider the terms in the limit  $s \rightarrow \infty$ . As we generically have the scaling  $v_s^{\text{eff}} \sim s^{-1}$ ,  $\rho_s^{\text{tot}} \sim s^{-1}$  and  $\mu_s^{\text{dr}} \sim s^2$  in any finite-temperature  $1/\beta$  equilibrium state, the term in the sum is finite at large  $s$  (as opposed to non-isotropic chains, where  $v_s^{\text{eff}} \sim e^{-c \cdot s}$ ), and therefore we define the chiral mode, coupling non-trivially to magnetization, as

$$\kappa \phi(x, t) = \frac{-1}{2\chi} \lim_{s \rightarrow \infty} \int_0^\infty du \left[ \rho_s^{\text{tot}}(u) v_s^{\text{eff}}(u) \mu_s^{\text{dr}} \right]_\beta [\delta n_s(u; x, t) - \delta n_s(-u; x, t)]. \quad (12)$$

Now let us consider the current of this mode. We have, using GHD Euler equations,  $\partial_t \delta n_s = -v_s^{\text{eff}} \partial_x \delta n_s$ ,

$$\partial_t \phi(x, t) = -\partial_x \left[ \frac{-1}{2\chi \kappa} \lim_{s \rightarrow \infty} \int_0^\infty du \left[ \rho_s^{\text{tot}}(u) (v_s^{\text{eff}}(u))^2 \mu_s^{\text{dr}} \right]_\beta [\delta n_s(u; x, t) + \delta n_s(-u; x, t)] \right]. \quad (13)$$

Therefore the current of  $\phi$  is given by

$$j_\phi = \frac{-1}{2\chi \kappa} \lim_{s \rightarrow \infty} \int_0^\infty du \left[ \rho_s^{\text{tot}}(u) (v_s^{\text{eff}}(u))^2 \mu_s^{\text{dr}} \right]_\beta [\delta n_s(u) + \delta n_s(-u)]. \quad (14)$$

In order to perform mode decoupling of this current we must expand it at second order in fluctuations, by perturbing each term in  $\left[ \rho_s^{\text{tot}}(u) (v_s^{\text{eff}}(u))^2 \mu_s^{\text{dr}} \right]_\beta$  around a thermal state. Indeed, at first order we can see that the expression gives zero after taking the limit, as  $\left[ \rho_s^{\text{tot}}(u) (v_s^{\text{eff}}(u))^2 \mu_s^{\text{dr}} \right]_\beta \sim 1/s$ . We obtain

$$j_\phi = \frac{1}{\pi \kappa \chi} \left( \lim_{s \rightarrow \infty} \int_0^\infty du \left[ (v_s^{\text{eff}}(u))^2 \mu_s^{\text{dr}} \right]_\beta [\delta n_s(u) + \delta n_s(-u)] \sum_{s'} \int_0^\infty du' \left[ m_{s'}^{\text{dr}} \rho_{s'}^{\text{tot}} \right]_\beta [\delta n_{s'}(u') + \delta n_{s'}(-u')] \right. \quad (15)$$

$$\left. + \lim_{s \rightarrow \infty} \int_0^\infty du \left[ (v_s^{\text{eff}}(u))^2 \rho_s^{\text{tot}} \right]_\beta [\delta n_s(u) + \delta n_s(-u)] \sum_{s'} \int_0^\infty du' \left[ \mu_{s'}^{\text{dr}} m_{s'}^{\text{dr}} \right]_\beta [\delta n_{s'}(u') + \delta n_{s'}(-u')] \right), \quad (16)$$

where one of the three terms of the expansion is zero due to antisymmetry of the velocity  $\int_0^\infty du \left[ (v_s^{\text{eff}}(u)) \rho_s^{\text{tot}} \mu_s^{\text{dr}} \right]_\beta [\delta n_s(u) + \delta n_s(-u)] = 0$ .

Now, under the general assumption that fluctuation of modes become almost independent of rapidity  $u$  at large  $s$  (due to  $v_s^{\text{eff}}(u) \sim \text{sgn}(u)/s$ ), namely as (with  $\Theta(u)$  the Heaviside step function)

$$\lim_{s \rightarrow \infty} \delta n_s(u; x, t) = \delta^{\text{R}}(x, t)\Theta(u) + \delta^{\text{L}}(x, t)\Theta(-u), \quad (17)$$

and, using that small strings are demagnetized, while large strings are asymptotically undressed, i.e.  $m_s^{\text{dr}} \rightarrow s$  at large  $s$  and  $m_s \sim 0$  at small  $s$ , we obtain

$$j_\phi = \frac{2\alpha}{\kappa\chi\pi}(\delta^{\text{R}} + \delta^{\text{L}})^2, \quad (18)$$

with the quantity

$$\alpha = \lim_{s \rightarrow \infty} \int_0^\infty du \left[ s (v_s^{\text{eff}}(u))^2 \rho_s^{\text{tot}}(u) \mu_s^{\text{dr}} \right]_\beta, \quad (19)$$

being well defined. The magnetization fluctuations can instead be expressed using  $|m| = \lim_{s \rightarrow \infty} \int_0^\infty du \rho_s^{\text{tot}}(u)$ , so that

$$(\delta m)^2 = \lim_{s \rightarrow \infty} \int_0^\infty du' \left[ s \rho_s^{\text{tot}}(u') \right]_\beta [\delta n_s(u') + \delta n_s(-u')] \int_0^\infty du \left[ s \rho_s^{\text{tot}}(u) \right]_\beta [\delta n_s(u) + \delta n_s(-u)] = \chi(\delta^{\text{R}} + \delta^{\text{L}})^2, \quad (20)$$

where we used  $\lim_{s \rightarrow \infty} \int_0^\infty du \left[ s \rho_s^{\text{tot}}(u) \right]_\beta = \sqrt{\chi}$ . In conclusion we find the following dependences on fluctuations (with  $\zeta = \lim_{s \rightarrow \infty} \int_0^\infty du \left[ \rho_s^{\text{tot}}(u) v_s^{\text{eff}}(u) \mu_s^{\text{dr}} \right]_\beta$ )

$$m^2 = \chi(\delta^{\text{R}} + \delta^{\text{L}})^2, \quad \phi = -\frac{\zeta}{\kappa}(\delta^{\text{R}} - \delta^{\text{L}}), \quad j_\phi = \frac{2\alpha}{\kappa\chi\pi}(\delta^{\text{R}} + \delta^{\text{L}})^2. \quad (21)$$

We thus conclude that from GHD and asymptotic mode decoupling, we have the Euler scale currents

$$j_m = \kappa m \phi, \quad j_\phi = \frac{2\alpha}{\pi\kappa\chi^2} m^2. \quad (22)$$

Adding noise and dissipative terms, we find the NLFH equations studied in the main text, with susceptibilities given by

$$\langle m^2 \rangle = \chi \quad \langle \phi^2 \rangle = \frac{\zeta^2}{\kappa^2}. \quad (23)$$

---

[1] B. Doyon, SciPost Physics Lecture Notes (2020), 10.21468/scipostphyslectnotes.18.

[2] J. De Nardis, M. Medenjak, C. Karrasch, and E. Ilievski, Phys. Rev. Lett. **123**, 186601 (2019).
